# Supplementary material for: Intrinsically knotted graphs and connected domination
Source: arXiv:2407.09476 ancillary file (2024-07-12)
Supplement: Supplementary file 1 [file Appendix1.pdf]

$$g_{10} = \{\{1, 3\}, \{1, 6\}, \{1, 7\}, \{1, 8\}, \{1, 9\}, \{1, 12\}, \{1, 15\}, \{2, 4\}, \{2, 7\}, \{2, 8\}, \{2, 9\}, \{2, 10\}, \{2, 13\}, \{2, 15\}, \{3, 5\}, \{3, 8\}, \{3, 9\}, \{3, 10\}, \{3, 11\}, \{3, 15\}, \{4, 6\}, \{4, 9\}, \{4, 10\}, \{4, 11\}, \{4, 12\}, \{4, 14\}, \{4, 15\}, \{5, 7\}, \{5, 10\}, \{5, 11\}, \{5, 12\}, \{5, 13\}, \{6, 8\}, \{6, 11\}, \{6, 12\}, \{6, 13\}, \{7, 9\}, \{7, 12\}, \{7, 13\}, \{7, 14\}, \{7, 15\}, \{8, 10\}, \{8, 13\}, \{8, 14\}, \{9, 11\}, \{9, 14\}, \{10, 12\}, \{10, 14\}, \{11, 13\}, \{11, 15\}, \{13, 14\}, \{14, 15\}\};$$

$$g_{11} = \{\{1, 3\}, \{1, 6\}, \{1, 7\}, \{1, 8\}, \{1, 9\}, \{1, 12\}, \{1, 15\}, \{2, 4\}, \{2, 7\}, \{2, 8\}, \{2, 9\}, \{2, 10\}, \{2, 13\}, \{2, 15\}, \{3, 5\}, \{3, 8\}, \{3, 9\}, \{3, 10\}, \{3, 11\}, \{3, 14\}, \{3, 15\}, \{4, 6\}, \{4, 9\}, \{4, 10\}, \{4, 11\}, \{4, 12\}, \{4, 15\}, \{5, 7\}, \{5, 10\}, \{5, 11\}, \{5, 12\}, \{5, 13\}, \{5, 14\}, \{6, 8\}, \{6, 11\}, \{6, 12\}, \{6, 13\}, \{7, 9\}, \{7, 12\}, \{7, 13\}, \{7, 14\}, \{7, 15\}, \{8, 10\}, \{8, 13\}, \{9, 11\}, \{9, 15\}, \{10, 12\}, \{10, 14\}, \{11, 13\}, \{11, 14\}, \{11, 15\}, \{12, 14\}, \{13, 14\}\};$$

$$g_{12} = \{\{1, 3\}, \{1, 6\}, \{1, 7\}, \{1, 8\}, \{1, 9\}, \{1, 12\}, \{1, 15\}, \{2, 4\}, \{2, 7\}, \{2, 8\}, \{2, 9\}, \{2, 10\}, \{2, 13\}, \{3, 5\}, \{3, 8\}, \{3, 9\}, \{3, 10\}, \{3, 11\}, \{3, 15\}, \{4, 6\}, \{4, 9\}, \{4, 10\}, \{4, 11\}, \{4, 12\}, \{4, 14\}, \{5, 7\}, \{5, 10\}, \{5, 11\}, \{5, 12\}, \{5, 13\}, \{5, 15\}, \{6, 8\}, \{6, 11\}, \{6, 12\}, \{6, 13\}, \{7, 9\}, \{7, 12\}, \{7, 13\}, \{7, 14\}, \{8, 10\}, \{8, 13\}, \{8, 14\}, \{8, 15\}, \{9, 11\}, \{9, 14\}, \{9, 15\}, \{10, 12\}, \{10, 14\}, \{10, 15\}, \{11, 13\}, \{11, 15\}, \{13, 14\}\};$$

$$g_{13} = \{\{1, 2\}, \{1, 4\}, \{1, 5\}, \{1, 10\}, \{1, 11\}, \{1, 13\}, \{1, 14\}, \{2, 3\}, \{2, 5\}, \{2, 6\}, \{2, 11\}, \{2, 12\}, \{2, 14\}, \{3, 4\}, \{3, 6\}, \{3, 7\}, \{3, 12\}, \{3, 13\}, \{3, 14\}, \{3, 15\}, \{4, 5\}, \{4, 7\}, \{4, 8\}, \{4, 13\}, \{5, 6\}, \{5, 8\}, \{5, 9\}, \{5, 14\}, \{6, 7\}, \{6, 9\}, \{6, 10\}, \{6, 14\}, \{7, 8\}, \{7, 10\}, \{7, 11\}, \{8, 9\}, \{8, 11\}, \{8, 12\}, \{8, 15\}, \{9, 10\}, \{9, 12\}, \{9, 13\}, \{9, 15\}, \{10, 11\}, \{10, 13\}, \{11, 12\}, \{11, 14\}, \{11, 15\}, \{12, 13\}, \{12, 15\}, \{13, 15\}, \{14, 15\}\};$$

$$g_{14} = \{\{1, 2\}, \{1, 4\}, \{1, 5\}, \{1, 10\}, \{1, 11\}, \{1, 13\}, \{1, 14\}, \{2, 3\}, \{2, 5\}, \{2, 6\}, \{2, 11\}, \{2, 12\}, \{2, 14\}, \{2, 15\}, \{3, 4\}, \{3, 6\}, \{3, 7\}, \{3, 12\}, \{3, 13\}, \{3, 14\}, \{4, 5\}, \{4, 7\}, \{4, 8\}, \{4, 13\}, \{4, 14\}, \{4, 15\}, \{5, 6\}, \{5, 8\}, \{5, 9\}, \{5, 15\}, \{6, 7\}, \{6, 9\}, \{6, 10\}, \{6, 14\}, \{6, 15\}, \{7, 8\}, \{7, 10\}, \{7, 11\}, \{7, 15\}, \{8, 9\}, \{8, 11\}, \{8, 12\}, \{8, 14\}, \{9, 10\}, \{9, 12\}, \{9, 13\}, \{9, 14\}, \{10, 11\}, \{10, 13\}, \{11, 12\}, \{12, 13\}, \{12, 15\}, \{13, 15\}\}.$$
